# Supplementary material for: Relativistic Calculation of Energies, Transition Parameters Hyperfine Structure, Land\'e g$_J$ and Isotope shifts factors for Ar$^{7+}$, Kr$^{25+}$ and Xe$^{43+}$ ions
Source: arXiv:2207.10179 source file (2022-07-20)
Supplement: Supplementary file 1 [file Tables.tex]

\documentclass[10pt]{article}
\usepackage{lscape}
\usepackage{booktabs}
\usepackage{longtable}
\usepackage{subfloat}
\usepackage[T1]{fontenc}
\textwidth = 15truecm
\textheight = 24 truecm
\hoffset = -2 truecm
\voffset = -2 truecm
\begin{document}
%\begin{landscape}
%\setcounter{table}{8}
%\setcounter{table}{0}
%\renewcommand\thetable{\Alph{}\arabic{table}}
\setcounter{tocdepth}{1}
%\alph{counter}
%\Alph{counter}
%
\setlength{\tabcolsep}{8pt}
\renewcommand\thetable{S1}
% [inline block 0: 9 envs, 297685 chars -> data_tex | \begin{longtable}{|c|c|c|c|c|c|c|c|} \caption{The present RCI E1 radiative wavelengths ($\lambda\;$(\AA)), transition ra...]

\end{landscape}
\end{document}
